# Supplementary material for: High detectivity terahertz radiation sensing using frequency-noise-optimized nanomechanical resonators
Source: arXiv:2401.16503 source file (2024-10-15)
Supplement: Supplementary file 1 [file Supplementary.pdf]

# Supplementary

### S1. Fractional frequency noise spectral density in angular frequency $S_y(\omega)$

In this paper we express $S_y(f)$ in units of $\mathrm{Hz}^{-1}$ to match the commonly used unit for noise equivalent power NEP ($\mathrm{W}/\sqrt{\mathrm{Hz}}$). However, in the context of mechanical oscillator (i.e., resonator), frequency noise is often expressed as $S_y(\omega)$ in angular frequency $\mathrm{rad/s}^{-1}$. Below, we provide the relevant equations for $S_y(\omega)$. Thermomechanical noise in $\mathrm{rad/s}^{-1}$ is given by [20]:

$$S_{y,TM}(\omega) = \frac{k_B T}{m_{eff}\omega_r^3 Q A_{rss}^2}|H_{mech}(\omega)|^2 \tag{S1}$$

where $H_{mech}(\omega) = 1/(1 + j\omega\tau_{mech})$. Thermal fluctuation in $\mathrm{rad/s}^{-1}$ is given by [16]:

$$S_{y,TF}(\omega) = \frac{2k_B T^2\alpha^2}{\pi G}|H_{th}(\omega)|^2 \tag{S2}$$

where $H_{th}(\omega) = 1/(1 + j\omega\tau_{th})$.

### S2. Transformation from fractional frequency noise spectral density $S_y(f)$ to Allan deviation $\sigma_A$

The theoretical Allan deviation plots in Fig. 1(b) are computed by evaluating the following integral:

$$\sigma_A(\tau) = \frac{\sqrt{2}}{\pi\tau}\left[\int_{-\infty}^{\infty}\frac{\mathrm{Sin}^4(\pi\tau f)}{f^2}S_y(f)\,df\right]^{\frac{1}{2}}. \tag{S3}$$

Note that in Fig. 1(b), Allan deviations limited by thermomechanical noise $\sigma_{A,TM}$ and thermal fluctuation noise $\sigma_{A,TF}$ are plotted by plugging Eq. (3-4) into Eq. (S3) accordingly. To solve Eq. (S3) numerically, we particularly use the built-in <integrate. quad> function in SciPy library with minimum absolute error tolerance (10E-30) to ensure solution accuracy.

### S3. Scaling Noise Equivalent Power NEP parameters with SiN membrane resonator sizes

In Fig. 1(c), we plotted SiN membrane resonators noise equivalent power NEP as a function of resonator side length $L$ for a 90 nm-thick SiN membrane by dimensionally scaling all parameters in the following equation Eq. (1). We begin by scaling all parameters (i.e., $m_{eff}, f_r, Q, \tau_{mech}, G, \tau_{th}$) in $S_{y,TM}(f)$ and $S_{y,TF}(f)$ (refer to Eq. (2-3)) with $L$. For parameters in $S_{y,TM}(f)$, we first scale the effective mass of square SiN membrane resonator $m_{eff}$ with $L$ by [20]:

$$m_{eff} = \frac{1}{4}L^2 t\rho, \tag{S4}$$

where $t = 90$ nm is membrane thickness and $\rho = 2900\ \mathrm{kg/m^3}$ is SiN material density. We then scale the resonance frequency $f_r$ according to $m_{eff}$ by [24]:

$$f_r = \frac{1}{4}\sqrt{\frac{\sigma(m^2+n^2)t}{m_{eff}}}, \tag{S5}$$

where $\sigma = 100$ MPa is the membrane built-in tensile stress, $m$ and $n$ are vibrational mode index in which for fundamental mode, $m = n = 1$. To scale SiN membrane resonator Q-factor with its side length $L$, we assume a typical Q-factor of 1 million for a $L = 3$ mm SiN membrane [15,16] and then scale Q-factor linearly with $L/t$, due to the dominant contribution of edge shape in dissipation dilution for membranes [23]. After scaling Q-factor and $f_r$ with $L$, we can thereafter use these two parameters to obtain the mechanical time constant $\tau_{mech}$ using $Q/(f_r\pi)$.

For parameters in $S_{y,TF}(f)$, note that the temperature coefficient of fractional frequency shift $\alpha$ purely depends on material constant, hence, remains the same when $L$ changes. We scale $G$ and $\tau_{th}$ according to $L$ using the closed-form heat transfer model presented in our previous work [5]. By scaling all aforementioned parameters in Eq. (1) with membrane side length $L$, we generate Fig. 1(c).

## S4. Defining the effective heat transfer area of SiN membrane resonator during terahertz absorption

We construct a volumetric heat transfer equation that includes linearized (i.e., assuming small temperature difference) radiative and solid-state conductive heat transfer to obtain membrane temperature profile $T_{SiN}$:

$$-k\nabla^2 T_{SiN} + \dot{q}_{rad} = \dot{q}_{absorb}. \tag{S6}$$

The full details of this heat transfer model is presented in [5]. We then use MATLAB built-in partial differential equation solver to solve Eq. (S4) in 2D. To account for localized, non-uniform terahertz absorption $\dot{q}_{absorb}$ of SiN membrane resonator, we use a rectangular pulse function in MATLAB. In specific, we set the width of the pulse to the effective diameter $D_{absorb} = 1$ mm of the terahertz metasurface absorber and the amplitude of the pulse to an arbitrary value to represent terahertz power absorption.

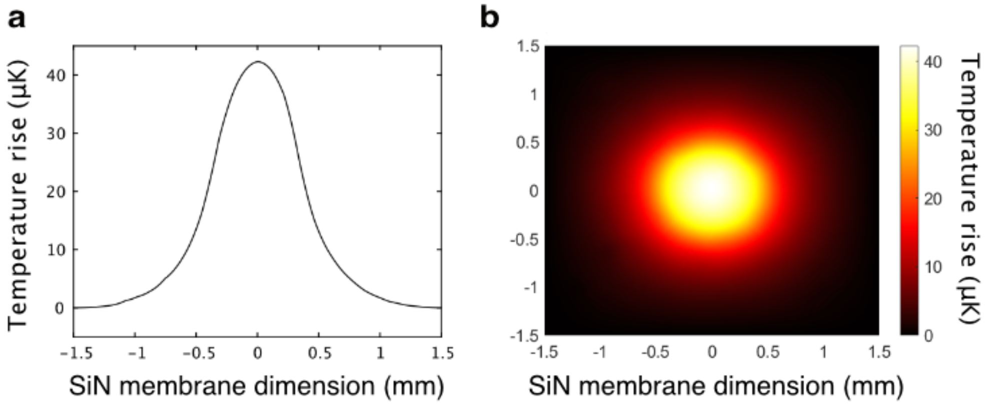


Fig. S1. (a) Interpolation of 2D temperature profile in 1D. (b) 2D temperature profile of SiN membrane when absorbing 1 nW radiation.

After solving Eq. (S6), we obtain temperature profile (see Fig. S1. a) of the SiN membrane during terahertz absorption. Therefore, the effective diameter of heating area ($D_{heating} \approx 2.2$ mm) can be extracted from this simulation. Note that $D_{heating}$ is mainly affected by SiN membrane internal solid-state conduction (i.e., thermal conductivity and thick of SiN) and effective absorbing diameter $D_{absorb}$, thus, independent of SiN membrane side length $L$ and $\dot{q}_{absorb}$. Inferring from the effective heating area $A_{heating} = \frac{\pi D_{heating}^2}{4} = 3.5\ \text{mm}^2$. Since all solid-state heat transfer is confined within $A_{heating}$, we can estimate subsequent thermal conductance $G \approx 4.4 \times 10^{-6}$ W/K by solely considering radiation:

$$G = 8A_{heating}\sigma_{sb}\varepsilon_{SiN}T_{room}^3, \tag{S7}$$

where $\sigma_{sb}$ is Stefan-Boltzmann constant, $\varepsilon_{SiN}$ is the hemispherical total emissivity of SiN membrane of 90 nm thickness and $T_{room}$ is the room temperature. We can then use $G$ to estimate the theoretical thermal time constant $\tau_{th}$ of our SiN membrane resonator under localized THz radiation absorption by:

$$\tau_{th} = \frac{c_{p_{\mathrm{SiN}}}\rho_{\mathrm{SiN}}V_{\mathrm{SiN}} + c_{p_{\mathrm{Ti}}}\rho_{\mathrm{Ti}}V_{\mathrm{Ti}}}{G}, \tag{S8}$$

where $\rho_{\mathrm{SiN}} = 2900\ \mathrm{Kg/m^3}$ is the SiN membrane density, $c_{p_{SiN}} = 700\ \mathrm{J/kgK}$ is SiN membrane specific heat capacity, $V_{\mathrm{SiN}} = 3.4 \times 10^{-13}\ \mathrm{m^3}$ is the SiN membrane volume associated with $A_{heating}$, $\rho_{\mathrm{Ti}} = 4500\ \mathrm{Kg/m^3}$ is the titanium density, $c_{p_{\mathrm{Ti}}} = 500\ \mathrm{J/kgK}$ is the specific heat capacity of titanium, $V_{\mathrm{Ti}} = 2.3 \times 10^{-14}\ \mathrm{m^3}$ is the titanium volume. Eq. (S8) yields a $\tau_{th}$ of 170 ms which is in close agreement with our experimental $\tau_{th}$ of 200 ms. The 15% discrepancy can be due to uncertainties in documented SiN and Ti material properties values.

### S5. Estimating thermal responsivity *R* under localized heating

With the localized temperature profile $T_{\mathrm{SiN}}$ solved in S4, we can then calculate the in-plane stress variation profile upon localized heating $\sigma_r$ in cylindrical coordinate system using:

$$\sigma_r(r) = -\alpha E\left[\frac{1}{r^2}\int_0^r r\Delta T_{\mathrm{SiN}}(r)dr + \frac{1+\nu}{1-\nu}\cdot\frac{\overline{\Delta T_{\mathrm{SiN}}}}{2}\right], \tag{S9}$$

where $\Delta T_{\mathrm{SiN}} = T_{\mathrm{SiN}}(r) - T_{\mathrm{room}}$ and $\overline{\Delta T_{\mathrm{SiN}}}$ is the average temperature difference. After obtaining the stress variation profile, we can then solve the eigen value of following partial differential equation numerically in MATLAB to obtain SiN membrane resonance frequency $f_r$ upon a specific amount of localized heat absorption:

$$\frac{1}{r}\frac{\partial}{\partial r}\left((\sigma+\sigma_r)r\frac{\partial U(r,t)}{\partial r}\right) - \rho\frac{\partial^2 U(r,t)}{\partial t^2} = 0, \tag{S10}$$

where $U(r,t)$ represents the out-of-plane displacement of the membrane. We vary $\dot{q}_{absorb}$ in Eq. (S6) and record the corresponding fractional resonance frequency shift $\delta f/f_r$ in Eq. (S10) to simulate thermal responsivity $R$ under the condition of localized heating (i.e., $R = \frac{\delta f/f_r}{\delta P_{abs}}$).

### S6. Mechanical modes, Q-factors and demodulated signal amplitudes

| $f_r$ | Q-factor | Demodulation amplitude under 500 µV actuation signal |
|---|---|---|
| 39 kHz | 122,980 | 12 µV |
| 57 kHz | 210,116 | 11 µV |
| 79 kHz | 86,964 | 32 µV |
| 86.5 kHz | 281,126 | 180 µV |
| 103.5 kHz | 88,902 | 190 µV |
| 104.5 kHz | 115,326 | 8 µV |
| 124.45 kHz | 870,334 | 190 µV |
